# Supplementary material for: Data-centric Dynamic Partial Order Reduction
Source: arXiv:1610.01188 source file (2019-01-25)
Supplement: Supplementary file 1 [file appendix.tex]

%\section{Example}\label{sec:examples}

\section{Comparison with related work}\label{sec:mcr_comparison}

Here we make a comparison with related existing work that also attempts to perform an exploration of the trace space of a concurrent system
based on a trace partitioning that is coarser than the Mazurkiewicz partitioning.
We first mention some such existing work, and then provide a specific example for one of them.

\subsection{Partitionings coarser than Mazurkiewicz}
In the past, there have been attempts to devise enumerative explorations of the trace space.
with respect to trace equivalences which are coarser than the Mazurkiewicz equivalence.
We list here some of these works.
\begin{compactenum}
%\item In~\cite{McMillan95}
\item In~\cite{Wang08} the authors introduce the Peephole Partial-order Reduction, in which various transitions can be considered independent in some, but not all traces of the system. However, their approach utilizes a SAT/SMT solver to prune away redundant interleavings.
\item The work of~\cite{HUANG15} builds upon the theoretical model of maximal causality of~\cite{Serbanuta13}
to provide an enumerative exploration where every explored trace corresponds to a distinct maximal causal model which captures the largest possible set of causally equivalent executions. The construction of each such trace queries an SMT solver with Integer Difference Logic (IDL) constraints, which requires exponential time in the worst case. In contrast, our algorithm has polynomial worst-case complexity per trace.
Even though SMT solvers scale well in practice, the important theoretical question of coarsening the trace space with polynomial worst-case guarantees had remained open.
The experimental section of~\cite{HUANG15} also reports that the running time on larger instances is dominated by the time spent in the SMT procedure.
Additionally, the work of~\cite{HUANG15} has no guarantees regarding the number of times that a class will be visited. In the next subsection we outline an example where that work will visit the same class an exponential number of times.
\item In~\cite{Sousa15} the authors introduce the unfolding-based Partial-order Reduction, which relies on state caching and cutoff events to further prune the trace space, and is thus stateful.
\end{compactenum}

\subsection{An example of Maximal Causality Reduction~\cite{HUANG15} that leads to exponentially many discoveries of the same class}

Here we use a small example to illustrate that the MCR enumerative exploration of~\cite{HUANG15}
can explore more traces than our $\EnumExplore$. 

\input{fig_mcr_comparison}

Consider the program depicted in Figure~\ref{subfig:mcr_processes}.
We have two processes $\Process_1, \Process_2$, and two global variables $x,y$.
The first processes is $\Process_1=\Write_y^1 \Read_x^1$, and the second process is $\Process_2=\Write_x^2 \Read_y^2$.
Additionally, we let $\Write_x^0$ and $\Write_y^0$ denote the two initialization write events.

\begin{compactenum}
\item Initially, the process starts in node $a$ with an empty seed interleaving.
The process will generate two seed interleavings $\{b,c\}$, forcing $\Read_x^1$ to observe the value of $\Write_x^2$, and $\Read_y^2$ to observe the value of $\Write_y^1$, respectively.
\item When in $b$, the process will create the seed interleaving $\{d\}$, forcing $\Read_y^2$ to observe the value of $\Write_y^1$.
\item When in $c$, the process will create the seed interleaving $\{e\}$, forcing $\Read_x^1$ to observe the value of $\Write_x^2$.
\end{compactenum}
Hence, all traces represented in the leaves $\{d, e\}$ of the above tree have the same observation function (and thus all reads observe the same values).
In contract, the optimality of our algorithm guarantees that the exploration will never explore both $d$ and $e$.

The example can easily be generalized to one where the MCR will explore the same class exponentially many times.
The only principle necessary to make the example work is that different branches of the recursion can accumulate the same read-to-write observations in different order, leading to the same read-to-write observations overall.

\section{Missing Proofs}\label{sec:proofs}

\subsection{Proofs of Section~\ref{sec:mazurkiewicz}}\label{subsec:proofs_of_mazurkiewicz}

%\smallskip
%\obstoval*
\begin{proof}[Proof of Lemma~\ref{lem:obs_to_val}]
The proof is by induction on the prefixes of $\Trace_1$.
We show inductively that for every $0\leq \ell \leq |\Trace_1|$, for all global events $\Event\in \Events{\Trace_1[\ell]}$ 
we have that if $\Event\in \Events{\Trace_2}$ then $\Value_{\Trace_1}(\Read)=\Value_{\Trace_2}(\Read)$.
Note that in the case where $\Event=\Read$ is a read event, then $\Read\in \Events{\Trace_2}$ follows directly from $\Obs_{\Trace_1}\subseteq \Obs_{\Trace_2}$.
The claim is true for $\ell=0$, since in that case $\Trace_1[\ell]=\eps$ and no event appears in $\Trace_1[\ell]$.
Now assume that the claim holds for all prefixes $\Trace_1[j]$ for $0\leq j\leq \ell$, and let 
\[
\Event=\arg\min_{\Event'\in \Events{\Trace_1}\setminus\Events{\Trace_1[\ell]}} \Index_{\Trace_1}(\Event')
\]
be the next global event in $\Trace_1$.
We distinguish two cases based on the type of $\Event$.
\begin{itemize}
\item $\Event=\Write\in \SysWrites$ is a write event of the form $g\gets \mathsf{write}~f(v_1,\dots,v_{n_i})$,
such that $\Process_i=\Proc(\Write)$.
Then the value of each local variable $v_j$ equals some $\alpha_j=\Value_{\Trace_1}(\Read_j)$, with $\Index_{\Trace_1}(\Read_j)\leq \ell$,
and by the induction hypothesis we have $\Read_j\in \Events{\Trace_2}$ and $\Value_{\Trace_1}(\Read_j)=\Value_{\Trace_2}(\Read_j)=\alpha_j$.
Since $\Process_i$ is deterministic, it easily follows that if $\Write\in \Events{\Trace_2}$ then
\begin{align*}
\Value_{\Trace_2}(\Write) &= f(\Value_{\Trace_1}(\Read_1),\dots, \Value_{\Trace_1}(\Read_{n_i}))\\
&= f(\alpha_1,\dots, \alpha_{n_i})= f(\Value_{\Trace_2}(\Read_1),\dots, \Value_{\Trace_2}(\Read_{n_i}))\\
& =\Value_{\Trace_1}(\Write)
\end{align*}

\item $\Event=\Read\in \SysReads$ is a read event, and let $\Write=\Obs_{\Trace_1}(\Read)$.
Let $\Process_i=\Proc(\Write)$, and since $\Process_i$ is deterministic, it easily follows from the induction hypothesis that $\Read\in\Events{\Trace_2}$,
and moreover that $\Value_{\Trace_1}(\Write)=\Value_{\Trace_2}(\Write)$.
Since $\Obs_{\Trace_2}(\Read)=\Write$, we have that 
\[
\Value_{\Trace_2}(\Read)=\Value_{\Trace_2}(\Write)=\Value_{\Trace_1}(\Write)=\Value_{\Trace_1}(\Read)
\]
The desired result follows.
\end{itemize}
\end{proof}

\subsection{Proofs of Section~\ref{sec:annotations}}\label{subsec:proofs_of_annotation}
%\smallskip
%\annotationbasis*
\begin{proof} [Proof of Lemma~\ref{lem:annotation_basis}]
\begin{compactenum}
\item Assume that $\Annotationpos$ has two distinct bases $(\SeqTrace_i)_i$ and $(\SeqTrace'_i)_i$.
Since each sequential trace corresponds to a deterministic computation of the corresponding process using $\Value_{\Annotationpos}$ as the value function of global events, we have that each $\SeqTrace_i$ and $\SeqTrace'_i$ share a prefix relationship (i.e., one is prefix of the other). Since the two basis are distinct, for some $j$ we have that one of $\SeqTrace_j$ and $\SeqTrace'_j$ is a proper prefix of the other.
Assume w.l.o.g. that $\SeqTrace'_j$ is a strict prefix of $\SeqTrace_j$.
Then replacing $\SeqTrace_i$ with $\SeqTrace'_i$ in $(\SeqTrace_i)_i$ yields another basis, thus $\SeqTrace_i$ is not minimal, a contradiction.
\item First, testing the conditions of Item~\ref{item:acyclicity} and Item~\ref{item:lock_obs} of well-formedness can be done in $O(|\Annotationpos|)$ time.
We now outline the process of constructing the basis $(\SeqTrace_i)_i$.
As a preprocessing step, we compute for each process $\Process_i$ the unique event $\Event_i\in X_i$ which is maximal wrt the program structure $\PS$.
Note that if $\Event_i$ is not unique for each process, then $\Annotationpos$ is not well-formed.
This requires $O(|\Annotationpos|)$ time for all processes $\Process_i$, simply by iterating over all events in $X$.
Then, the unique basis $(\SeqTrace_i)_i$ can be constructed by executing each process locally, and using the value function $\Value_{\Annotationpos}$ for assigning values to global events.
The execution stops when $\Event_i$ is reached, and the constructed sequential trace $\SeqTrace_i$ is returned.
Finally, $(\SeqTrace_i)_i$ constitute a basis of $\Annotationpos$ if the conditions~(a) and~(b) of Item~\ref{item:basis} of well-formedness are met,
which can be done in $O(n)$ time.
\item It follows easily from Remark~\ref{rem:annotationpos_value} and the above construction that if $\Trace$ realizes $\Annotationpos$,
then $\Annotationpos$ must be well-formed and $\Trace\in \SeqTrace_1\Conv\dots \Conv \SeqTrace_k$.
\end{compactenum}
\end{proof}

%\smallskip
%\aea*
\begin{proof}
[Proof of Lemma~\ref{lem:aea}]
The proof is by reduction from \SATMONOTONE~\cite[LO4]{Garey79}.
In \SATMONOTONE, the input is a propositional 3CNF formula $\phi$ in which every literal is positive,
and the goal is to decide whether there exists a satisfying assignment for $\phi$ that assigns exactly one literal per clause to $\True$.

The reduction proceeds as follows.
In the following, we let $C$ and $D$ range over the clauses and $x_i$ over the variables of $\phi$.
We assume w.l.o.g. that no variable repeats in the same clause.
For every variable $x_i$, we introduce a node $\Write'_i\in V$.
For every clause $C=(x_{C_1}\lor x_{C_2} \lor x_{C_3})$, we introduce a pair of nodes $\Write^C_{C_j}, \Read^C_{C_j}\in V$
and an edge $(\Write^C_{C_j}, \Read^C_{C_j})\in E$, where $j\in \{1,2,3\}$.
Additionally, we introduce an edge $(\Write^C_{C_j}, \Write'_{C_l})\in E$ for every pair $j,l\in\{1,2,3\}$ such that $j\neq l$,
and an edge $(\Write'_{C_j}, \Read^C_{C_l})$ for each $j\in \{1,2,3\}$, where $l=( j+1) \mod 3 + 1$.
Finally, for every pair of clauses $C, D$ and $l_1,l_2\in \{1,2,3\}$ such that $C_{l_1}=D_{l_2}=\ell$
(i.e., $C$ and $D$ share the same variable $x_{\ell}$ in positions $l_1$ and $l_2$),
we add edges $(\Write^{C}_{\ell}, \Read^{D}_{\ell}), (\Write^{D}_{\ell}, \Read^{C}_{\ell})\in E$.
The set $H$ consists of triplets of nodes $(\Write'_{C_j},\Write^C_{C_j},\Read^C_{C_j})$ for every clause $C$ and $j\in\{1,2,3\}$.
Figure~\ref{fig:reduction} illustrates the above construction.

Let $X$ be an edge addition set that solves \AEA~on input $(G,H)$ and note that for every pair of triplets
$(\Write'_{i},\Write^C_{i},\Read^C_{i}), (\Write'_{i},\Write^D_{i},\Read^D_{i})\in H$, we have that
$(\Write'_{i},\Write^C_{i}) \in X$ iff $(\Write'_{i},\Write^D_{i})\in X$,
i.e., for every node $\Write'_i$, the set $X$ contains either only all incoming, or only all outgoing edges of $\Write'_i$ specified by $H$.
To see this, observe that if there exists such a pair of triplets with $(\Write'_{i},\Write^C_{i}), (\Read^D_{i}, \Write'_{i})\in H$,
then $G_X=(V,E\cup X)$ would contain the cycle
\[
\Write'_{i} \to \Write^C_{i} \to \Read^D_{i} \to \Write'_{i}
\]
which contradicts that $X$ is a solution to the problem.
Given such an edge addition set $X$, we obtain an assignment on the variables of $\phi$ by setting $x_i=\True$ iff $X$ contains an edge $(\Write'_{C_j},\Write^C_{C_j})$ for some clause $C$ and $j\in \{1,2,3\}$.
By the previous remark, the assignment of values to variables of $\phi$ is well-defined.

It is easy to verify that the construction takes polynomial time in the size of $\phi$.
In the following, we argue that the answer to \SATMONOTONE~is true iff the answer to \AEA~is also true.

\smallskip
$(\Rightarrow)$. Let $X$ be a solution to \AEA~on $(G,H)$, and we argue that every clause $C$ of $\phi$ contains exactly one variable set to $\True$. Indeed, $C$ contains at least one such variable, otherwise $G_X$ would contain a cycle
\[
\Read^C_{C_1}\to \Write'_{C_1} \to \Read^C_{C_2}\to \Write'_{C_2} \to \Read^C_{C_3}\to \Write'_{C_3} \to \Read^C_{C_1}
\]
Similarly, $C$ contains at most one variable of $C$ set to $\True$, as two such variables $x_i, x_j$ would imply that $G_X$ contains a cycle
\[
\Write'_i\to \Write^C_{i} \to \Write'_j \to \Write^C_{j}\to \Write'_i
\]

\smallskip
$(\Leftarrow)$. Consider any satisfying assignment of $\phi$, and construct an edge addition set $X=\{e_i\}_i$ such that 
for each triplet $(\Write'_{i},\Write^C_{i},\Read^C_{i})\in H$ we have
\[
e_i = 
\left\{\begin{array}{rl}
        (\Write'_i, \Write^C_i), &\text{if } x_i=\True\\
        (\Read^C_i, \Write'_i), &\text{if } x_i=\False        
\end{array}
\right.
\]
Given a clause $C$, we denote by $V_C=\bigcup_{i=1}^3\{\Write'_{C_i},\Write^C_{C_i}, \Read^C_{C_i}\}$,
and by $G_X\restr{V_C}$ the subgraph of $G_X$ restricted to nodes in $V_C$.
We now argue that $G_X$ does not contain a cycle.
Assume towards contradiction otherwise, and let $\mathcal{C}$ be such a cycle.
\begin{compactenum}
\item If $\mathcal{C}$ contains a node of the form $\Write^C_{C_j}$ for some $j\in \{1,2,3\}$ then $\mathcal{C}$ traverses the edge 
$(\Write'_{C_j}, \Write^C_{C_j})$, and thus $x_{\ell}$ is assigned $\True$, where $\ell=C_j$
Since $G_X$ contains no edge of the form $(\Read^D_{\ell}, \Write'_{\ell})$ for any clause $D$,
$\mathcal{C}$ must traverse an edge $(\Write^D_{D_i}, \Write'_{\ell})$ for some clause $D$.
Hence there is a first node $\Write^D_{D_i}$ traversed by $\mathcal{C}$ after $\Write^C_{\ell}$, for some clause $D$ and $i\in\{1,2,3\}$
and thus $G_X$ contains an edge $(\Write'_{D_i},\Write^D_{D_i})$, and hence $x_l$ is assigned $\True$,
where $l=D_i$.
By our choice of $\Write^D_{D_i}$, the node $\Write'_{D_i}$ can only be reached via the edge $(\Read^{D}_{D_i}, \Write'_{D_i})$,
which requires that $x_l$ is assigned $\False$, a contradiction.

\item If $\mathcal{C}$ contains no node of the form $\Write^C_{C_j}$, then it must be a cycle in $G\restr{V_C}$, for some clause $C$.
The only such cycle that traverses no $\Write^C_{C_j}$ can be
\[
\Read^C_{C_1}\to \Write'_{C_1} \to \Read^C_{C_2}\to \Write'_{C_2} \to \Read^C_{C_3}\to \Write'_{C_3} \to \Read^C_{C_1}
\]
which requires that all $x_{C_i}$ are assigned $\False$, for each $i\in\{1,2,3\}$, which contradicts that $C$ has a variable assigned $\True$.
\end{compactenum}
The desired result follows.
\end{proof}

%\smallskip
%\aatoann*
\begin{proof} 
[Proof of Lemma~\ref{lem:aatoann}]
We present both directions of the proof.
\begin{compactitem}
\item $(\Rightarrow)$. Let $\Trace$ be any trace that realizes $\Annotationpos$.
Observe that for any edge $(u,v)\in E$ we have $\Index_{\Trace}(\Event(u))< \Index_{\Trace}(\Event(v))$, since $\PS(\Event(u), \Write_{u,v})$ and $\PS(\Read_{u,v}, \Event(v))$ and $\Annotationpos(\Read_{u,v})=\Write_{u,v}$.
Additionally, $\Trace$ satisfies that either $\Index_{\Trace}(\Write'_i)<\Write_{\Trace}(\Write_i)$, or $\Index_{\Trace}(\Read_i)<\Write_{\Trace}(\Write'_i)$. 
In the former case we an edge $(x_i, y_i)$, and in the latter case we add $(z_i, x_i)$ in an edge set $X$.
Since $\Trace$ induces a total order on the vertices of $G$, $G_X$ is acyclic, and thus $X$ is an edge addition set for $(G,H)$.
\item $(\Leftarrow)$. If $X$ is an edge addition set for $(G,H)$ then $G_X$ is acyclic and any topological order of the vertices of $G_X=(V, E\cup X)$ induces a trace that realizes $\Annotationpos$.
\end{compactitem}
The desired result follows.
\end{proof}

\smallskip
\smallskip
\begin{restatable}{lemma}{realize}\label{lem:realize}
Given a well-formed positive annotation $\Annotationpos$ over a basis $(\SeqTrace_i)_i$, $\Realize$ constructs a trace $\Trace$ that realizes $\Annotationpos$ (or concludes that $\Annotationpos$ is not realizable) and requires $O(n^3)$ time, where $n=\sum_i|\SeqTrace_i|$.
\end{restatable}
\begin{proof} We present the correctness proof and complexity analysis.

\noindent{\em Correctness.}
We first argue about correctness.
\begin{compactenum}
\item If $\Realize$ returns a sequence of events $\Trace$ (Line~\ref{line:return_trace}) then clearly $\Trace$ is a trace since $\Trace$ respects the program structure $\PS$ (Line~\ref{line:fact}), and by the definition of the well-formed annotation, lock semantics are respected (i.e., critical regions protected by locks do not overlap).
Additionally, $\Trace$ realizes $\Annotationpos$,  as the sequential consistency axioms are satisfied because of Line~\ref{line:annotation} and Line~\ref{line:fact}.

\item If $\Annotationpos$ is realizable by a trace $\Trace$, then $\Trace$ is a linearization of $E^*$, thus for every pair of distinct conflicting events $(\Event_1,\Event_2)\in E^*$ we have $\Index_{\Trace}(\Event_1)<\Index_{\Trace}(\Event_2)$ (Line~\ref{line:fact}). By the sequential consistency axioms, for every pair $(\Read, \Write)\in \Annotationpos$ and $\Write'\neq \Write$ with $\Confl(\Read,\Write')$ we have either $\Index_{\Trace}(\Write')<\Index_{\Trace}(\Write)$ or $\Index_{\Trace}(\Read)< \Index_{\Trace}(\Write')$ (Line~\ref{line:annotation}).
Finally, since $\Trace$ induces a total order on $V$, it is clearly transitive (Line~\ref{line:transitivity}) and antisymmetric (Line~\ref{line:antisymmetry}).
Hence the set of 2SAT clauses $\mathcal{C}$ is satisfiable.
It suffices to argue that $G'=(V',E')$ (Line~\ref{line:topological_order}) is acyclic, as then any topological order of $G'$
will satisfy the sequential consistency axioms (Line~\ref{line:annotation}).
Assume towards contradiction otherwise.
If $G^*$ has a cycle, then $\Annotationpos$ is not realizable, as $\Trace$ must linearize $E^*$. Hence $G^*$ must be acyclic,
Thus, any cycle $C$ in $G'$ traverses an edge $(\Event_1,\Event_2)\in E'\setminus E^*$, hence $f(x_{\Event_1,\Event_2})=\True$.
We distinguish the following cases.
\begin{compactenum}
\item If there exists a cycle $C$ which traverses a single edge $(\Event_1,\Event_2)\in E'\setminus E^*$, then there is a path $\Event_2\Path \Event_1$ traversing only edges of $E^*$. Since $E^*$ is transitively closed, we have that $(\Event_2,\Event_1)\in E^*$ and hence $f(x_{\Event_2,\Event_1})=\True$ (Line~\ref{line:fact}). Thus, by antisymmetry, $f(x_{\Event_1,\Event_2})=\False$ (Line~\ref{line:antisymmetry}), a contradiction.
\item Otherwise, let $C$ be a simple cycle in $G^*$ that traverses the fewest number of edges in $E'\setminus E^*$,
and $C$ must traverse at least two edges $(\Event_1,\Event_2), (\Event_3, \Event_4)\in E'\setminus E^*$.
Observe that $\Proc(\Event_1)\neq \Proc(\Event_2)$ and $\Proc(\Event_3)\neq \Proc(\Event_4)$
as otherwise we would have $(\Event_2,\Event_1)\in E^*$ or $(\Event_4,\Event_3)\in E^*$,
and there would exist a cycle that traverses a single edge from $E'\setminus E^*$
(namely, $\Event_1\to\Event_2\to \Event_1$ or $\Event_3\to\Event_4\to\Event_3$).
Since $\System$ is acyclic, by construction (Line~\ref{line:variables}) $|\{\Proc(\Event_1), \Proc(\Event_2), \Proc(\Event_3), \Proc(\Event_4)\}|=2$,
i.e., there exist two processes $\Process_i$, $\Process_j$ such that 
\begin{align*}
&\Event_1\in \SysEvents_i  \text{ and } \Event_2\in\SysEvents_j \text{ and }\\
&\Event_3, \Event_4\in \SysEvents_i\cup \SysEvents_j  \text{ and }  \Event_3, \Event_4\not \in \SysEvents_i\cap \SysEvents_j
\end{align*}

Then $C$ traverses an edge $(\Event'_3, \Event'_4)$ such that either $\Event'_3=\Event_1$ or $\PS(\Event'_3, \Event_1)$,
and either $\Event_2=\Event'_4$ or $\PS(\Event_2, \Event'_4)$.
In all cases, we have $(\Event'_3, \Event_1), (\Event_2, \Event'_4)\in E^*$.
Since $(\Event'_3, \Event'_4)\in E'$ we have $f(x_{\Event'_3, \Event'_4})=\True$, and by transitivity (Line~\ref{line:transitivity}), we have that $f(x_{\Event_2,\Event_1})=\True$, a contradiction.
\end{compactenum}
\end{compactenum}

\noindent{\em Complexity.}
%%We now turn our attention to complexity.
The transitive closure requires $O(n^3)$ time, since $|V|=n$.
The set $V_{\mathcal{C}}$ (Line~\ref{line:variables}) has $O(n^2)$ variables and each of the loops for constructing clauses iterates over triplets of nodes, hence the 2SAT instance is constructed in $O(n^3)$ time.
Computing a satisfying assignment for $\mathcal{C}$ (or concluding that none exists) requires linear time in $|\mathcal{C}|$~\cite{Tarjan79}, hence this step costs $O(n^3)$.
Finally, constructing $G'$ and computing a topological sorting of its vertices requires $O(n^2)$ time in total.
The desired result follows.
\end{proof}

\subsection{Proofs of Section~\ref{sec:enumerative}}\label{subsec:enumerative}

%\smallskip
%\inevitable*
\begin{proof}[Proof of Lemma~\ref{lem:obs_to_enable_max}]
We argue that every event $\Event'\in\Past_{\Trace_1}(\Event)\cup \{\Event\}$ is inevitable in $\Trace_2$.
Let $\Trace'_2$ be any lock-free maximal extension of $\Trace_2$.
Assume towards contradiction that $(\Past_{\Trace_1}(\Event)\cup \{\Event\})\setminus\Events{\Trace'_2}\neq \emptyset$, and let
\[
\Event_m=\arg\min_{\Event'\in (\Past_{\Trace_1}(\Event)\cup \{\Event\})\setminus\Events{\Trace'_2}}\Index_{\Trace_1}(\Event')
\]
be the first such event in $\Trace_1$, and let $\Process_i=\Proc(\Event_m)$ be the process of $\Event_m$.
By Remark~\ref{rem:causal_past}, for every event $\Event'\in\Past_{\Trace_1}(\Event_m)$ we have $\Event'\in \Past_{\Trace_1}(\Event)$, and since $\Index_{\Trace_1}(\Event')<\Index_{\Trace_1}(\Event_m)$, we have $\Event'\in \Events{\Trace'_2}$.
Let $(x,y)$ be the edge of $\CFG_i$ labeled with $\Event_m$.
Since $\Event'\in \Events{\Trace'_2}$, the program counter of $\Process_i$ becomes $x$ at some point in $\Trace'_2$.
We examine the number of outgoing edges from node $x$.
\begin{enumerate}
\item If $x$ has one outgoing edge, we distinguish whether $\Event_m$ is a lock-acquire event or not.
\begin{enumerate}
\item If $\Event_m$ is not a lock-acquire event, then $\Event_m$ is always enabled after $\Event'$ in $\Trace'_2$, hence $\Trace'_2$ is not maximal, a contradiction.
\item If $\Event_m: \mathsf{acquire~} l$, since $\Trace'_2$ is a lock-free trace, $l$ is released in $\State(\Trace'_2)$,
hence $\Event_m\in\Enabled(\Trace'_2)$ and $\Trace'_2$ is not maximal, a contradiction.
\end{enumerate}
\item If $x$ has at least two outgoing edges then $\Event_m$ is of the form $\Event_m:~b_j(v_1,\dots,v_{n_i})$, where $v_i\in\Locals_i$ are local variables of $\Process_i$.
Let $\Trace_{\Event_m}=\Trace_2'\Project \Past_{\Trace_1'}(\Event_m)$.
Since for every read $\Read\in \Past_{\Trace_1}(\Event)$ we have $\Read\in \Events{\Trace_2}$ and $\Obs_{\Trace_1}(\Read)=\Obs_{\Trace_2}(\Read)$, by Remark~\ref{rem:causal_past}, the same holds for reads $\Read\in \Past_{\Trace_1}(\Event_m)$, i.e.,  for every read $\Read\in \Past_{\Trace_1}(\Event_m)$ we have $\Read\in \Events{\Trace_2}$ and $\Obs_{\Trace_1}(\Read)=\Obs_{\Trace_2}(\Read)$.
It is easy to see that additionally $\Read\in\Events{\Trace_{\Event_m}}$ and $\Obs_{\Trace_1}(\Read)=\Obs_{\Trace_{\Event_m}}(\Read)$.
Thus, we have $\Obs_{\Trace_{\Event_m}}\subseteq \Obs_{\Trace_1}$.
By Lemma~\ref{lem:obs_to_val}, we have $\Value_{\Trace_{\Event_m}}(\Read)=\Value_{\Trace_1}(\Read)$ for every read $\Read$,
and since $\Process_i$ is deterministic, the value of $v$ on $x$ is a function of those reads, and thus each $v_i$ has the same value
when the program counter of $\Process_i$ reaches node $x$ in $\Trace_1$ and $\Trace'_2$.
Since $\Event_m$ appears in $\Trace_1$, $\Event_m$ is always enabled after $\Event'$ in $\Trace'_2$, hence $\Trace'_2$ is not maximal, a contradiction.
\end{enumerate}
The desired result follows.
\end{proof}
\begin{proof}[Proof of Lemma~\ref{lem:compactness}]
Examine the recursion tree $\RecTree$ generated by $\EnumExplore$, where every node $u$ is labeled with the trace $\Trace_{u}$ and annotation input $\Annotation_u=(\Annotationpos_u, \Annotationneg_u)$ given to $\EnumExplore$.
Let $x$ and $y$ be the nodes that correspond to inputs $(\Trace_1, \Annotation_1)$ and $(\Trace_1,\Annotation_2)$ respectively,
and we argue that $\Annotation_{x}\neq \Annotation_{y}$.
If $x$ is an ancestor of $y$, then when $\EnumExplore$ was executed on input $(\Trace_x,\Annotation_x)$,
a read $\Read$ created $\Annotationpos_{\Read,\Write}$ in Line~\ref{line:strengthenpos} on the branch from $x$ to the direction of $y$ in $\RecTree$, with the property that $\Read\not \in \Domain(\Annotationpos_x)$.
Since the algorithm never removes pairs $(\Read, \Write)$ from the positive annotations, we have that $(\Read,\Write)\in \Annotation_{y}$,
hence $\Annotation_{x}\neq \Annotation_{y}$.
A similar argument holds if $y$ is an ancestor of $x$.
Now consider the case that $x$ and $y$ do not have an ancestor-descendant relationship.
Let $z$ be the lowest common ancestor of $x$ and $y$ in $\RecTree$,
and $z_x$ (resp. $z_y$) the child of $z$ in the direction of $x$ (resp. $y$).
Let $\Read_x$ (resp. $\Read_y$) be the read on Line~\ref{line:strengthenpos} that generated
$\Annotationpos_{z_x}$ (resp. $\Annotationpos_{z_y}$), i.e.,
\[
\Annotationpos_{z_x}=\Annotationpos_{z}\cup \{(\Read_x, \Write_x)\} \quad \text{and} \quad \Annotationpos_{z_y}=\Annotationpos_{z}\cup \{(\Read_y, \Write_y)\}
\]
If $\Read_x=\Read_y=\Read$ then $\Write_x\neq \Write_y$, thus $\Annotationpos_{z_x}(\Read)\neq \Annotationpos_{z_y}$,
and since the algorithm never removes pairs $(\Read,\Write)$ from positive annotations we have that
$\Annotation_{x}\neq \Annotation_{y}$.
Now assume that $\Read_x\neq \Read_y$, and w.l.o.g. that $\Index_{\Trace_j}(\Read_x)< \Index_{\Trace_j}(\Read_y)$.
Then, before $\EnumExplore(\Annotation_{z_y})$ is executed, Line~\ref{line:strengthenneg} adds $\Write_x\in \Annotationneg(\Read_x)$.
Since the algorithm never removes entries from the negative annotation, by Line~\ref{line:strengthenpos}, we have that $(\Read_x,\Write_x)\not \in \Annotationpos_y$. 
%Observe that $\Write_x\neq \Obs_{\Trace_z}(\Read_x)$, whereas in every node $u$ that is either $z_y$ or some descendant of $z_y$,
%if $\Read_x\in \Events{\Trace}$ then 
%\begin{compactenum}
%\item if $\Read_x$ is added in $\Annotationpos_u$ belonging to the causal past of some mutation pair $(\Read, \Write)$, we have that $\Annotationpos_u(\Read_x)=\Obs_{\Trace_z}(\Read_x)\neq \Write_x$, and
%\item if $\Read_x$ is added in $\Annotationpos_u$ as part of a mutation pair $(\Read_x, \Write)$, then by the condition on the negative annotation of \cref{line:foreachwrite}, we have that $\Write\neq \Write_x$.
%\end{compactenum}
In all cases we have $\Annotation_{x}\neq\Annotation_{y}$, as desired.
\end{proof}

%\smallskip
%\completeness*
\begin{proof}[Proof of Lemma~\ref{lem:completeness}]
Let $\RecTree$ be the recursion tree of $\EnumExplore$.
Given a node $u$ of $\RecTree$, we denote by $\Trace_u$ and $\Annotation_u=(\Annotationpos_u, \Annotationneg_u)$ the input of $\EnumExplore$ on $u$. Since $\Trace_u$ is always a maximal extension of a trace returned by procedure $\Realize$ on input $\Annotationpos_u$, by Lemma~\ref{lem:realize} we have that $\Trace_u$ is compatible with $\Annotationpos_u$, thus it suffices to show
that $\EnumExplore$ is called with a positive annotation being equal to $\Obs$.
We define a traversal on $\RecTree$ with the following properties:
\begin{compactenum}
\item\label{item:agreement} If $u$ is the current node of the traversal, then $\Annotationpos_u\subseteq \Obs$.
\item\label{item:progress} If  $\Annotationpos_u\subset \Obs$, then the traversal proceeds either
\begin{compactenum}
\item\label{item:child} to a node $v$ of $\RecTree$ with $\Annotationpos_u\subset \Annotationpos_v$,
\item\label{item:other} to some other node of $\RecTree$,
\end{compactenum}
and Item~\ref{item:other} happens a finite number of times.
\end{compactenum}
Observe that every time the traversal executes Item~\ref{item:child}, $\Obs$ agrees with
$\Annotationpos_v$ on more reads than $\Annotationpos_u$.
Since Item~\ref{item:other} is executed a finite number of times, any such traversal is guaranteed to reach a node $w$ with $\Annotation_w=\Obs$. 

The traversal starts from $u$ being the root of $\RecTree$,
and Item~\ref{item:agreement} holds as then $\Annotationpos_u=\emptyset\subseteq \Obs$.
Now consider that the traversal is on any node $u$ that satisfies Item~\ref{item:agreement}.
Since $\Trace_u$ is a maximal extension of a trace returned by procedure $\Realize$ on input $\Annotationpos_u$, Lemma~\ref{lem:realize} guarantees that $\Trace_u$ is a maximal trace that realizes $\Annotationpos_u$.
Let $\Trace^{*}$ be a trace that realizes $\Obs$, and $\Read$ be the first read of $\Trace^{*}$ not in $\Annotationpos_u$, i.e.,
\[
\Read=\arg\min_{\Read'\in \Events{\Trace^{*}}\setminus\Domain(\Annotationpos_u)} \Index_{\Trace^{*}}(\Read')
\]
and $\Write=\Obs_{\Trace^{*}}(\Read)$.
Then for every $\Read'\in \Past_{\Trace^{*}}(\Read)$, we have $\Index_{\Trace^{*}}(\Read')<\Index_{\Trace^{*}}(\Read')$
and thus $\Read'\in \Events{\Trace_u}$ and $\Obs_{\Trace^{*}}(\Read')=\Obs_{\Trace_u}(\Read')$.
By Lemma~\ref{lem:obs_to_enable_max}, we have $\Read\in \Events{\Trace_u}$.
Since $\Index_{\Trace^{*}}(\Write)<\Index_{\Trace^{*}}(\Read)$, a similar argument yields that $\Write\in \Events{\Trace_u}$.
We now distinguish two cases, based on whether $\Write\in \Annotationneg_u(\Read)$ or not.
\begin{compactenum}
\item If $\Write\not \in \Annotationneg_u(\Read)$, then in Line~\ref{line:get_trace} the algorithm will generate a trace $\Trace'$ that is compatible with the strengthened annotation $\Annotationpos_u\cup(\Read, \Write)$, and call itself recursively on some child $v$ of $u$
with $\Annotationpos_v=\Annotationpos_u\cup(\Read, \Write)$.
The traversal proceeds to $v$ and Item~\ref{item:agreement} holds, as desired.

\item If $\Write\in \Annotationneg_u(\Read)$, 
then there exists a highest ancestor $x$ of $u$ in $\RecTree$ where $\EnumExplore$ was called with
$(\Read, \Write)\in \Annotationneg_x$.
Following Line~\ref{line:strengthenneg}, this can only have happened if 
$x$ has a sibling $v$ in $\RecTree$ with $(\Read, \Write)\in \Annotationpos_v$.
Let $z$ be the parent of $x,v$, and we have $\Annotationpos_z\subset \Annotationpos_u\subset \Obs$,
and $\Annotationpos_v=\Annotationpos_z \cup (\Read,\Write)\subseteq \Obs$.
Thus, the traversal proceeds to $v$ and Item\ref{item:agreement} holds, as desired.
In this case, we say that the traversal \emph{backtracks to $x$ through $z$}.
\end{compactenum}

Finally, we argue that Item~\ref{item:other} will only occur a finite number of times in the traversal.
Since $\RecTree$ is finite, it suffices to argue that the traversal backtracks through any node $z$ a finite number of times.
Indeed, fix such a node $z$ and let $x_1,x_2,\dots$ be the sequence of (not necessarily distinct) children of $z$ that the traversal backtracks to, through $z$.
Let $\Read_i$ be the unique read in $\Domain(\Annotationpos_{x_i})\setminus\Domain(\Annotationpos_{z})$.
By Line~\ref{line:foreachread}, we have that $\Index_{\Trace_z}(\Read_{i+1}) < \Index_{\Trace_z}(\Read_i)$, hence no node repeats in the sequence $(x_i)_i$,
and thus the traversal backtracks through $z$ a finite number of times.
The desired result follows.
\end{proof}

%\smallskip
%\enumexplore*
\begin{proof}[Proof of Theorem~\ref{them:enum_explore}]
Lemma~\ref{lem:compactness} and Lemma~\ref{lem:completeness} guarantee the optimality of $\EnumExplore$, 
i.e., that $\EnumExplore$ explores each class of $\TraceSpace/\sim_{\Obs}$ exactly once.
The time spent in each class is the time for attempting all possible mutations on the witness trace $\Trace$
which is the trace used by the algorithm to explore the corresponding observation function.
There are at most $n^2$ such mutations, and according to Theorem~\ref{them:annotation}, 
each such mutation requires $O(n^3)$ time to be applied (or conclude that $\Trace$ cannot be mutated in the attempted way).
The desired result follows.
\end{proof}

\subsection{Proofs of Section\ref{sec:cyclic_architectures}}\label{subsec:proofs_of_cyclic}

%\smallskip
%\obsrefined*
\begin{proof}[Proof of Lemma~\ref{lem:obs_refined}]
By Theorem~\ref{them:annotation}, we have $\Trace_1\sim_{\Obs}\Trace_2$.
Consider any pair of distinct write events $\Write_1,\Write_2\in \Writes{\Trace_1}\cap (\SysWrites_i \cup \SysWrites_j)$
with $\Location(\Write_1)=\Location(\Write_2)=g$ and $g\in \Weight_{\System}(\Process_i, \Process_j)$,
and observe that $\Write_1$ and $\Write_2$ are dependent.
Hence, we have $\HB{\Write_1}{\Trace_1}{\Write_2}$ iff $\HB{\Write_1}{\Trace_2}{\Write_2}$,
and thus $\Index_{\Trace_1}(\Write_1)< \Index_{\Trace_1}(\Write_2)$ iff $\Index_{\Trace_2}(\Write_1)< \Index_{\Trace_2}(\Write_2)$,
as desired.
\end{proof}

\smallskip
\begin{restatable}{lemma}{realizemodified}
\label{lem:realize_modified}
Given a well-formed positive annotation $\Annotationpos$ over a basis $(\SeqTrace_i)_i$,
and the modified communication graph $G'_{\System^X}=(V_{\System^X}, E_{\System^X}\setminus X, \Weight_{\System^X})$,
$\Realize$ constructs a trace $\Trace$ that realizes $\Annotationpos$ (or concludes that $\Annotationpos$ is not realizable)
and requires $O(n^3)$ time, where $n=\sum_i|\SeqTrace_i|$.
\end{restatable}
\begin{proof}[(Sketch)]
First, note that due to the new locks $\ObservedLocks$, $\Annotationpos$ already induces a total order on the lock-acquire and lock-release events that access the same lock $l_g\in \ObservedLocks$.
Hence $\Annotationpos$ already induces a total order between the write events that are protected by the same lock $l_g\in \ObservedLocks$.
Thus, given the basis $(\SeqTrace_i)_i$, $\Annotationpos$ is realizable iff that total order respects $\Annotationpos$, 
and there is a way to order the remaining pairwise dependent events between pairs of processes $(\Process_i, \Process_j)\not \in X$, such that the ordering respects the sequential consistency axioms.
The crucial property is that since $X$ is an all-but-two cycle set of $G_{\System}$,
the transitivity (Line~\ref{line:transitivity}) and antisymmetry (Line~\ref{line:antisymmetry}) clauses ensure that a satisfying assignment preserves acyclicity of the graph $G'$ constructed in Line~\ref{line:topological_order}.
The complexity analysis is similar to Lemma~\ref{lem:realize}.
\end{proof}

%\enumexplorecyclic*
\begin{proof}[Proof of Theorem~\ref{them:enum_explore_cyclic}]
We argue that $\EnumExploreCyclic$ is then optimal for the cyclic architecture $\System$ wrt the equivalence $\sim_{\Obs}^X$.
\begin{compactenum}
\item (\emph{Compactness}). 
For any two distinct positive annotations $\Annotationpos_1$, $\Annotationpos_2$ examined by $\EnumExplore$ when exploring the trace space of $\System^X$, Lemma~\ref{lem:compactness} guarantees that $\Annotationpos_1\neq \Annotationpos_2$.
Let $\Trace_1$ and $\Trace_2$ be the traces returned by $\Realize$ on inputs $\Annotationpos_1$ and $\Annotationpos_2$ respectively.
Assume that $\Trace_1$ is not a prefix of $\Trace_2$ (the argument is similar if $\Trace_2$ is not a prefix of $\Trace_1$, and since $\Annotationpos_1\neq \Annotationpos_2$, it is not the case that each is a prefix of the other).
This implies that at least one of the following holds.
\begin{compactenum}
\item There is a read event $\Read\in \Events{\Trace_1}$ such that $(\Read, \Obs_{\Trace_1}(\Read))\not \in \Obs_{\Trace_2}$,
in which case two different classes of $\sim_{\Obs}$ are explored. Since $\sim_{\Obs}^X$ refines $\sim_{\Obs}$ it follows that two different classes of $\sim{\Obs}^X$ are explored.
\item There is a lock-acquire event $\Event_a\in \Events{\Trace_1}$ such that  $(\Event_a, \Obs_{\Trace_1}(\Event_a))\not \in \Obs_{\Trace_2}$.
In this case, the write event $\Write$ protected by the lock-acquire event $\Event_a$ either does not appear $\Trace_2$ or there exists a conflicting write event $\Write'$ in $\Trace_1$ such that $\Trace_1$ and $\Trace_2$ are ordered differently in $\Trace_1$ and $\Trace_2$.
Hence the two annotations $\Annotationpos_1$ and $\Annotationpos_2$ are used to explore different classes of $\sim_{\Obs}^X$.
\end{compactenum}
\item (\emph{Completeness}). 
Lemma~\ref{lem:realize_modified} together with the completeness statement of Lemma~\ref{lem:completeness} guarantees that for every observation function $\Obs$ of the trace space of $\System^X$, there is an annotation function $\Annotationpos$ used by $\EnumExplore$ such that $\Obs=\Annotationpos$.
Since the lock-acquire and lock-release events are read and write events respectively,
any two traces which have a different order on a pair of write events $\Write$, $\Write'$ such that $\Write$ and $\Write'$ are protected by observable locks, will also be explored.
\end{compactenum}
Finally, the maximum size of a trace in $\System$ is asymptotically equal to the maximum size of a trace in $\System^X$,
from which the complexity bound follows.
\end{proof}
